# Supplementary material for: Can ChatGPT Enable ITS? The Case of Mixed Traffic Control via Reinforcement Learning
Source: arXiv:2306.08094 source file (2023-09-25)
Supplement: Supplementary file 1 [file appendix.tex]

\section*{APPENDIX}

\subsection{Conflict resolution mechanism}
